# Supplementary material for: Automatic Co-Registration of Aerial Imagery and Untextured Model Data Utilizing Average Shading Gradients
Source: arXiv:1906.10882 source file (2019-09-21)
Supplement: Supplementary file 1 [file 08_appendix.tex]

\section*{APPENDIX (Optional)}\label{Asec:appendix}

Any additional supporting data may be appended, provided the paper does not exceed the limits given above.
